# Supplementary material for: Data-Efficient Learning from Human Interventions for Mobile Robots
Source: arXiv:2503.04969 source file (2025-03-06)
Supplement: Supplementary file 1 [file appendix.tex]

\newpage
\section*{Appendix}

\section{Building Reactive Traffic Scenario}
\label{sec:turn_to_environment}
In this section, we introduce the scenario importing pipeline built upon a recent lightweight driving simulator~\cite{li2021metadrive}.
The simulator MetaDrive supports accurate physics simulation, multiple sensory inputs, and a flexible interface to customize maps and run the simulation efficiently. All of this makes MetaDrive an ideal platform for TrafficGen's scenario-importing pipeline.

\noindent \textbf{Importing Road Network}.
As discussed in 
Sec.~3
, we define a traffic scenario as a tuple of HD map and traffic flow.
The first step to instantiate a reactive driving environment is to import the road map into the simulator so that the vehicle can navigate to a specific point.

The basic road structure is represented by 3D polylines and polygons.
Since the lane centers and lane lines are represented by a list of points in Waymo Open Dataset~\cite{waymo_open_dataset}, we can approximate the lane by building a set of lane fragments and adding a rigid body and visual appearance for them. 
Therefore, each lane has its Frenet-coordinates.
The local coordinates can be used to localize vehicles, computing their distance to the left and right boundaries and determining whether a given object is on the lane.
The lane line such as yellow solid line and broken white line can also be rebuilt in the virtual world in a similar way.
Therefore contacts between vehicle and lane line can be detected to trigger some events like yielding cost or terminating the training if driving on yellow solid line.

For global routing, we build a road graph based on the connectivity information provided by Waymo dataset~\cite{waymo_open_dataset} to support route searching algorithms like BFS. With the routing and localization information, vehicles can follow the searched reference route to the destination and freely drive in the drivable region. 

\noindent \textbf{Importing Traffic Flow}.
The outputs of our model are state sequences of generated vehicles. Instead of synchronizing vehicles' positions and headings recorded in data frame-by-frame, we additionally apply a rule-based IDM policy~\cite{kesting2010enhanced} to actuate a vehicle following the generated path to its destination, enabling interactive behavior like deceleration, yielding, and emergency stop. These IDM vehicles utilize lidar to detect surrounding vehicles. If there are vehicles on the future trajectory of the target vehicle, the target vehicle will automatically determine the speed according to IDM.
Therefore, these vehicles can react to the RL agent. 

\section{Procedural Generation Baseline}
\noindent\textbf{Procedural Generation.}
MetaDrive is able to generate numerous maps through Procedural Generation (PG). Concretely, there are several basic road structures such as intersections and roundabouts, which serve as building blocks for the search-based PG algorithm. Given different random seed, the PG algorithm then randomly combine these blocks and compose different maps. Also, each building block has unique randomizable parameters such as curvature of \textit{Curve block}, so that domain randomization can be applied to generate the same road structures but in different shapes. Therefore, all generated maps will be unique, given a unique random seed.
To generate traffic flow on these procedurally generated maps, several hand-crafted rules are first executed for approximating the real-world traffic distribution and spawning traffic vehicles in the simulated world. After initialization, these vehicles are actuated by IDM policy too and will navigate to the randomly assigned destinations. 

\noindent\textbf{Experiment result.}
The agents trained in PG scenarios are benchmarked on the real-world test set. The awful test success rate implies that in spite of meticulous hand-crafted traffic scenarios, the driving skills learned in these synthetic scenes can not be generalized to real-world scenarios.
This, in turn, points out that methods building traffic scenarios from real-world data, such as \textit{TrafficGen}, is promising for bridging the sim-to-real gap.

\section{Environment Details}
\label{appendix:env_details}
In the driving task, the objective of RL agents is to steer the target vehicles with low-level continuous control actions, namely acceleration, brake, and steering.

\noindent\textbf{Observation.}
The observation of RL agents is as follows:
\begin{itemize}[noitemsep, leftmargin=2em]
  \item A 240-dimensional vector denoting the Lidar-like point clouds with $50 m$ maximum detecting distance centering at the target vehicle. 
  Each entry is in $[0, 1]$ with Gaussian noise and represents the relative distance of the nearest obstacle in the specified direction.
  \item A vector containing the data that summarizes the target vehicle's state such as the steering, heading, velocity, and relative distance to the left and right boundaries.
  \item The navigation information that guides the target vehicle toward the destination. 
  We sparsely spread a set of checkpoints, 50m apart on average, in the route and use the relative positions toward future checkpoints as additional observation of the target vehicle. 
\end{itemize}

\noindent\textbf{Reward and Cost Scheme.}
The reward function is composed of four parts as follows:
\begin{equation}
\label{eq:reward-functgion}
  R = c_{1}R_{disp} + c_{2}R_{speed} + R_{term}.
\end{equation}
The \textit{displacement reward} $R_{disp} = d_t - d_{t-1}$, wherein the $d_t$ and $d_{t-1}$ denotes the longitudinal movement of the target vehicle in Frenet coordinates of the current lane between two consecutive time steps, provides a dense reward to encourage the agent to move forward. 
The \textit{speed reward} $R_{speed} = v_t/v_{max}$ incentives agent to drive fast. $v_{t}$ and $v_{max}$ denote the current velocity and the maximum velocity ($80 \ km/h$), respectively.
We also define a sparse \textit{terminal reward} $R_{term}$, which is non-zero only at the last time step. At that step, we set $R_{disp} = R_{speed} = 0$ and assign $R_{term}$ according to the terminal state.
$R_{term}$ is set to $+10$ if the vehicle reaches the destination, $-5$ for crashing others or violating the traffic rule.
We set $c_1 = 1$ and $c_2 = 0.1$.
For measuring safety, collision with vehicles, obstacles, and sidewalk raises a cost of $+1$ at each time step. The sum of cost generated in one episode is episode cost, a metric like an episode reward, but reflecting safety instead.

\noindent\textbf{Termination Conditions and Evaluation Metrics.} 
Since we attempt to benchmark the safety of trained agents, collisions with vehicles and the sidewalk will not terminate the episode. The episode will be terminated only when: 1) the agent drives out of the drivable area, such as driving outside of the yellow solid line, 2) the agent arrives at the destination and 3) the episode length exceeds the pre-defined horizon (1000 steps). 
For each trained agent, we evaluate it in 100 held-out test environments and define the ratio of episodes where the agent arrives at the destination as the \textit{success rate}. The \textit{Episodic Cost}, also referred to as \textit{Safety Violation} is the average episode cost on 100 test environments.
Since each agent are trained across 5 random seeds, this evaluation process will be executed for 5 agent which has the same training setting but different random seeds. We report the average and std on the 2 metrics mentioned above for measuring the performance and the safety of trained agents.

\noindent\textbf{Importing Scenarios.} 
Unlike the RL agent that can select new routes in the drivable area to the destination, 
Traffic vehicles follow the logged trajectories, while IDM is used~\cite{kesting2010enhanced, kesting2007general} for control speed so that they can react to RL agent which may behave differently from the logged ego car, performing behaviors like yielding and emergency stop.

\noindent\textbf{Statistical Results Processing.}
Since each agent is trained with 5 random seeds, the evaluation process will be executed for 5 agents which have the same training setting but different random seeds. We report the mean and std of the 2 aforementioned metrics to measure the performance and the safety of trained agents.

\section{Implementation Details}

\begin{table}[ht]
\centering
\centering
\label{hyper:tt}
\caption{TrafficGen}
\begin{tabular}{@{}ll@{}}
\toprule
Hyper-parameter             & Value  \\ \midrule
Feature Size              & 1024    \\
Training epochs   & 30     \\
Data Usage for Initializer & 50,000 \\
Data Usage for Actuator & 150,000 \\
Learning Rate   & $\expnumber{3}{-4}$ \\ 
Activation Function & ``relu'' \\
MLP Layers & 3\\
\bottomrule
\end{tabular}
\end{table}

\begin{table}[ht]
\centering
\centering
\caption{PPO}
\label{hyper:ppo}
\begin{tabular}{@{}ll@{}}
\toprule
Hyper-parameter             & Value  \\ \midrule
KL Coefficient              & 0.2    \\
$\lambda$ for GAE~\citep{schulman2018highdimensional} & 0.95 \\
Discounted Factor $\gamma$   & 0.99  \\
Number of SGD epochs   & 20     \\
Train Batch Size & 30,000 \\
SGD mini-batch size & 256 \\
Learning Rate   & $\expnumber{3}{-4}$ \\ 
Clip Parameter $\epsilon$ & 0.2 \\
Activation Function & ``tanh'' \\
MLP Hidden Units & 256 \\
MLP Layers & 2\\
\bottomrule
\end{tabular}
\end{table}

\label{appendix:resource_usage}
The training is executed on servers with 8 x Nivdia 1080ti and 256 G memory.
When training PPO agents, we use RLLib~\cite{liang2018rllib} and host 16 concurrent trials on 8 x Nvidia A100 GPU. Each trial consumes 6 CPUs with 10 parallel rollout workers. 
The total memory consumption for each trial is approximately 100 G. 

For the TrafficGen model, we set the feature dimension of $\mathbf{v'}$ to be 1024, and use 3-layer MLPs with hidden dimensions of [2048, 1024, 256] for attribute modeling. During training, we train both networks with a learning rate of $3e-4$ for 30 epochs.

Note that we make two assumptions about vehicles that are driving on the road. First, the distance between a vehicle and its nearest road center lane should be limited. We set the range limit to 5 meters in experiments. Second, the angle between a vehicle's heading and the road center lane's direction should be limited. We set the angle limit to $\pm 90^{\circ}$ in experiments. These assumptions help to filter out invalid vehicles in the dataset. Besides, they give good prior information for the model, ensuring that invalid vehicles such as the out-of-road and retrograde ones will not be generated.
